# Supplementary material for: Unifying and Personalizing Weakly-supervised Federated Medical Image Segmentation via Adaptive Representation and Aggregation
Source: arXiv:2304.05635 source file (2023-04-12)
Supplement: Supplementary file 2 [file appendix.pdf]

# Appendix 2418

Anonymous

Anonymous Organization

**Table A1.** Details of the datasets utilized in our experiments. Scribble<sup>2</sup> refers to scribbles of a different style generated using another automated algorithm.

| Modality | Site | Original Dataset     | Train-Test Sample Size | Annotation Type       | Processed Resolution [px] | Manufacturer                          |
|----------|------|----------------------|------------------------|-----------------------|---------------------------|---------------------------------------|
| Fundus   | A    | Drishti-G            | 50:51                  | Scribble              | 384×384                   | (Aravind eye hospital)                |
|          | B    | RIM-ONE-r            | 99:60                  | Scribble <sup>2</sup> |                           | Nidek AFC-210                         |
|          | C    | REFUGE-train         | 320:80                 | Bounding box          |                           | Zeiss Visucam 500                     |
|          | D    | REFUGE-val           | 320:80                 | Point                 |                           | Canon CR-2                            |
|          | E    | GAMMA                | 100:100                | Block                 |                           | KOWA camera & Topcon TRC-NW400        |
| OCTA     | A    | FAZID                | 244:60                 | Scribble              | 256×256                   | Cirrus 5000 Angioplex                 |
|          | B    | OCTA500-3M           | 150:50                 | Point                 |                           | RTVue-XR, Optovue, CA                 |
|          | C    | OCTA500-6M           | 200:100                | Block                 |                           | RTVue-XR, Optovue, CA                 |
|          | D    | OCTA-25K (sOCTA-3×3) | 708:304                | Bounding box          |                           | Triton DRI-OCT, Topcon Inc            |
|          | E    | ROSE                 | 30:9                   | Scribble <sup>2</sup> |                           | RTVueXR Avanti SD-OCT system, Optovue |

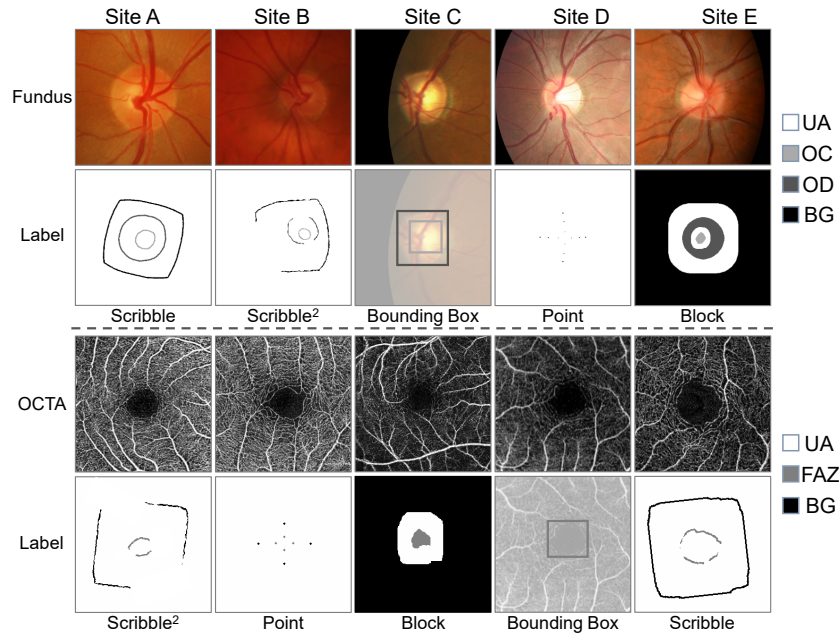

**Fig. A1.** Examples of the images and corresponding sparse annotations of each site. UA, OC, OD, FAZ, and BG represent unlabeled areas, optic cup, optic disc, foveal avascular zone, and background respectively.

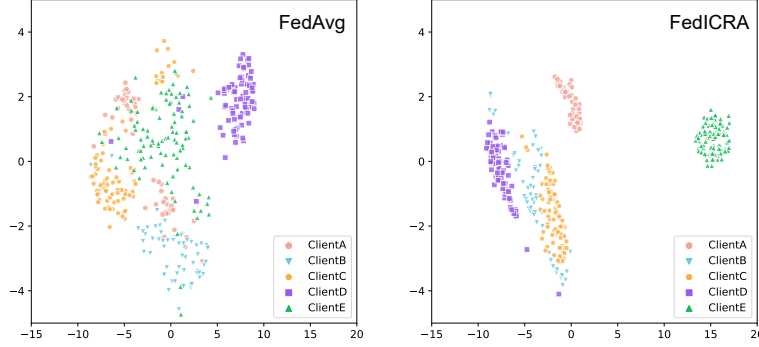

**Fig. A2.** Comparison of data embeddings on ODOC segmentation test sets via t-SNE visualization.

**Table A2.** Performance comparison (HD95) of different FL methods, local and centralized training settings on ODOC segmentation. The best results are highlighted in bold, and the second-best ones are underlined.

| Sites          | HD95 (OD) ↓      |                    |                  |                  |                   |              |  | HD95 (OC) ↓       |                   |                  |                  |                    |              |              | Overall |
|----------------|------------------|--------------------|------------------|------------------|-------------------|--------------|--|-------------------|-------------------|------------------|------------------|--------------------|--------------|--------------|---------|
|                | A                | B                  | C                | D                | E                 | Avg.         |  | A                 | B                 | C                | D                | E                  | Avg.         |              |         |
| FedAvg         | 13.17±8.04       | 24.10±26.68        | 9.28±7.23        | 20.80±43.31      | 24.59±33.12       | 18.39        |  | 18.56±12.99       | 23.98±28.08       | 11.19±9.99       | 22.42±47.48      | 16.80±32.37        | 18.59        |              | 18.49   |
| FedProx        | 8.38±4.17        | 15.72±21.67        | 10.64±14.23      | 16.02±27.82      | 20.36±31.30       | 14.22        |  | <b>14.17±6.91</b> | 12.82±7.34        | 13.36±13.58      | 13.91±25.36      | 16.10±30.24        | 14.07        |              | 14.15   |
| FT             | 10.07±8.96       | 22.26±25.08        | <b>8.51±7.58</b> | 40.12±53.19      | 20.36±31.19       | 20.26        |  | 19.96±12.44       | 22.24±27.52       | 11.68±9.94       | 31.60±51.63      | 14.59±26.15        | 20.02        |              | 20.14   |
| FedBN          | 8.78±4.77        | 18.06±28.02        | 19.54±32.51      | 10.72±25.22      | 17.68±28.85       | 14.96        |  | 15.70±7.14        | <b>12.08±6.79</b> | 17.24±32.24      | 9.96±24.07       | <u>11.96±13.18</u> | 13.39        |              | 14.17   |
| FedAP          | 9.19±6.18        | 21.59±14.86        | 8.96±12.14       | <b>5.77±2.61</b> | 16.80±29.82       | <u>12.46</u> |  | <u>15.09±7.47</u> | 14.68±19.84       | 12.66±14.05      | <u>7.05±3.19</u> | 14.49±25.30        | <u>12.91</u> | <u>12.69</u> |         |
| FedRep         | 17.39±28.48      | 21.59±27.13        | 23.56±34.86      | 54.10±68.55      | 31.00±39.85       | 29.53        |  | 27.61±37.21       | 18.90±21.65       | 17.89±29.64      | 50.60±79.80      | 17.71±28.70        | 26.54        |              | 28.03   |
| MetaFed        | 41.99±52.18      | 28.19±44.51        | 119.84±70.20     | 33.57±55.59      | 23.06±20.78       | 49.33        |  | 34.82±43.31       | 13.86±7.60        | 32.83±53.45      | 9.37±14.39       | 14.56±16.37        | 21.09        |              | 35.21   |
| FedICRA (Ours) | <b>7.86±4.76</b> | <b>11.65±19.33</b> | 8.52±9.44        | 7.70±8.26        | <b>8.59±12.66</b> | <b>8.87</b>  |  | 16.49±11.85       | 14.76±21.34       | <b>8.71±4.05</b> | <b>5.76±2.53</b> | <b>9.99±15.22</b>  | <b>11.14</b> | <b>10.01</b> |         |
| LT (Weak)      | 26.91±42.21      | 44.05±59.07        | 74.35±74.73      | 151.71±54.14     | 19.53±23.93       | 63.31        |  | 16.51±8.51        | 35.98±58.07       | 24.93±43.10      | 19.27±33.63      | 16.45±22.63        | 22.62        |              | 42.97   |
| CT (Weak)      | 9.32±5.86        | 12.25±7.00         | 7.29±3.23        | 11.97±15.68      | 14.52±23.10       | 11.07        |  | 15.55±7.30        | 13.79±7.13        | 10.73±4.32       | 9.83±16.04       | 12.15±19.02        | 12.41        |              | 11.74   |
| LT (Full)      | 9.27±10.42       | 6.26±4.83          | 7.55±6.05        | 5.38±2.63        | 11.07±20.82       | 7.91         |  | 13.34±7.13        | 12.62±8.56        | 9.18±5.43        | 6.30±3.48        | 11.51±16.56        | 10.59        |              | 9.25    |
| CT (Full)      | 6.40±3.48        | 8.95±7.34          | 6.13±2.53        | 4.62±2.01        | 8.92±18.19        | 7.00         |  | 12.31±5.45        | 11.28±6.95        | 8.47±4.47        | 5.74±2.70        | 8.48±11.91         | 9.26         |              | 8.13    |

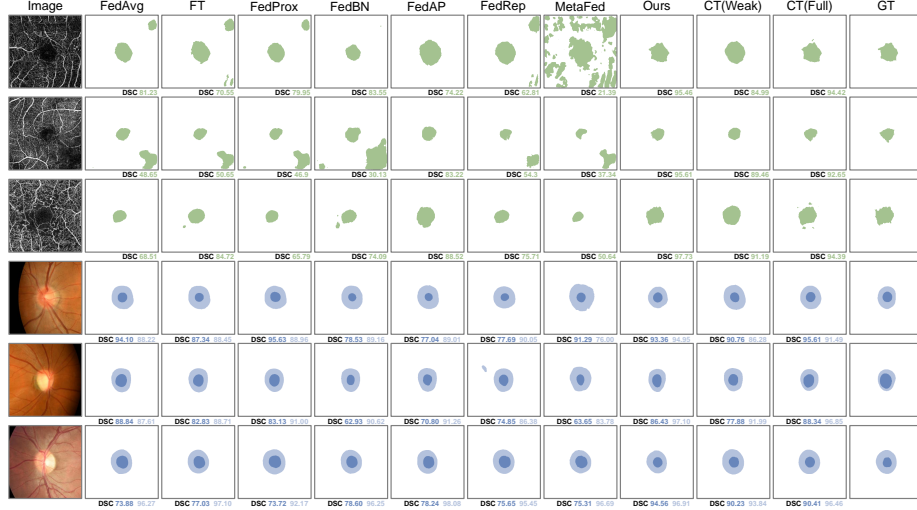

**Fig. A3.** Visualization results from FedICRA and other SOTA methods (CT indicates centralized training with **Weak** and **Full** respectively denoting utilizing sparse annotations and full masks).
